# Supplementary material for: Position paper: A systematic framework for categorising IoT device fingerprinting mechanisms
Source: arXiv:2010.08466 source file (2020-10-19)
Supplement: Supplementary file 1 [file appendix_abbreviations.tex]

\section{List of Abbreviations}

\begin{tabular}{ll}
\textbf{ML} & Machine Learning \\
\textbf{FPR} & False Positive Rate \\
\textbf{TPR} & True Positive Rate \\
\textbf{SVM} & Support Vector Machine\\
\textbf{k-NN} & k Nearest Neighbour \\
\end{tabular}
